# Supplementary material for: Toward Student-Oriented Teacher Network Training For Knowledge Distillation
Source: arXiv:2206.06661 source file (2024-05-09)
Supplement: Supplementary file 1 [file proof-for-presentation.tex]

%%% ----------- For presentation --------------------
$$
\begin{aligned}
\min -\frac{1}{N}\sum_{i=1}^{N} 1(y^{(i)}) \cdot \log \bm{p} = -\left(\frac{1}{N}\sum_{i=1}^{N} 1(y^{(i)}) \right) \cdot \log \bm{p} \\
s.t. \bm{1} \cdot \bm{p} = 1
\end{aligned}
$$

$f(x) = \bm{p}$

$x \sim P(X)$

$y \sim P(Y=y|x),~y=\{0, 1, \cdots, K-1\}$

$$
- \bm{q}\cdot \log \bm{q} \le -\bm{q}\cdot \log \bm{p},~\text{if}~\bm{1}\cdot \bm{p} = 1, \bm{1}\cdot \bm{q} = 1. 
$$

$$
\nabla_{\bm{p}} = - \frac{1}{N} \sum_{i=1}^N 1(y^{(i)}) \odot \frac{1}{\bm{p}} + \bm{1} = 0
$$

$$
\bm{p} = \frac{1}{N} \sum_{i=1}^N 1(y^{(i)})
$$

$$
\begin{aligned}
\min -\frac{1}{N}\sum_{i=1}^{N} 1(y^{(i)}) \cdot \log \bm{p}^{(i)} = - \frac{1}{N}\sum_{j=1}^{M} \sum_{i\in \mathcal{S}_j} 1(y^{(i)}) \cdot \log \bm{p}_j \\
s.t. \bm{1} \cdot \bm{p} = 1
\end{aligned}
$$

$\mathcal{S}_1$, $\mathcal{S}_2$, $\mathcal{S}_3$

$$
\nabla_{\bm{p_1}} = - \frac{1}{N} \sum_{i\in \mathcal{S}_1} 1(y^{(i)}) \odot \frac{1}{\bm{p}_1} + \bm{1} = 0
$$

$$
\bm{p}_1 = \frac{1}{N} \sum_{i\in \mathcal{S}_1} 1(y^{(i)})
$$

$$
\bm{p}_1 = \frac{1}{|\mathcal{S}_1|} \sum_{i\in \mathcal{S}_1} 1(y^{(i)})
$$

$$
P(Y=y|x^{(i)})
$$

$$
\begin{aligned}
\min -\frac{1}{N}\sum_{i=1}^{N} 1(y^{(i)}) \cdot \log \bm{p}^{(i)} = - \frac{1}{N}\sum_{j=1}^{M} \sum_{i\in \mathcal{S}_j} 1(y^{(i)}) \cdot \log \left(\bm{p}_j + \bm{\varepsilon}_j^{(i)}\right) \\
s.t. \bm{1} \cdot \bm{p} = 1
\end{aligned}
$$

$$
\bm{p}_1 = \left(\frac{1}{N} \sum_{i\in \mathcal{S}_1} 1(y^{(i)})\right)(1 + K\varepsilon) - \varepsilon
$$

$P(Y=y|z)$

$$
\frac{1}{N} \sum_{\{i|z\in \mathcal{Z}^{(i)}\}} P(Y=y|x^{(i)})
$$
