# Supplementary material for: Toward Student-Oriented Teacher Network Training For Knowledge Distillation
Source: arXiv:2206.06661 source file (2024-05-09)
Supplement: Supplementary file 2 [file 0-proof_removed.tex]

\section{Proofs}
\label{section:all-proof}

% \subsection{Proof of Lemma~\ref{lemma:sample-mean-relax}}
% \begin{proof}
% We first show a side result that generalizes Hoeffding's inequality to a category distribution.
% \begin{lemma}[Hoeffding's inequality to category distribution.]
% % \label{lemma:sample-mean}
% % Let i.i.d. samples $(x_i, y_i) \in \{(x,y)~ |~ \mathbf{p}^*(x) = \mathbf{q}\}$ and $i = 1, \cdots, N$. For any $p$-norm $\|\cdot\|$ and any $\varepsilon > 0$,  we have
% % \begin{equation}
% %     P\left(\left\|\frac{1}{N} \sum_{i=1}^N \mathbf{1}_{y_i} - \mathbf{q} \right\| \ge \varepsilon\right)  \le 2K\exp\left(-\frac{2N}{K^2}\varepsilon^2\right).
% % \end{equation}


% Let $\mathbf{p}_i \in \mathbb{R}^K,~i = 1,\cdots, N$ be a set of independent random variables with properties $\sum_k \mathbf{p}_i^k = 1$ and $\mathbf{p}_i^k \ge 0$, where $\mathbf{p}^k$ denote the $k$-th coordinate of a vector $\mathbf{p}$. Let $\mathbf{\bar{p}} = N^{-1} \sum_{i=1}^N \mathbf{p}_i$. Then for any $p$-norm $\|\cdot\|$ and any $\varepsilon > 0$,  we have
% \begin{equation}
%     P\left(\left\| \mathbf{\bar{p}} - \mathbb{E}\left[ \mathbf{\bar{p}} \right] \right\| \ge \varepsilon\right)  \le 2\exp\left(-\frac{N}{2K}\varepsilon^2\right).
% \end{equation}

% \end{lemma}

% \begin{proof}
% Note that a category distribution can be viewed as a special case of a multinomial distribution. We utilize the classic results on the concentration properties of multinomial distribution based on $\ell_1$ norm~\cite{Weissman2003InequalitiesFT, Qian2020ConcentrationIF}, namely
% \begin{equation}
% \label{eq:classic_bound}
% P(\left\| \mathbf{\bar{p}} - \mathbb{E}\left[ \mathbf{\bar{p}} \right] \right\|_1 \ge \varepsilon) \le 2\exp\left({-\frac{N}{2 K}\varepsilon^2}\right)
% \end{equation}

% % We have 
% % \begin{equation}
% %     \mathbf{\bar{p}}^k = \frac{1}{N}\sum_{i=1}^N \mathbf{p}_i^k
% % \end{equation} by the rule of vector summation.
% % Now by Hoeffding's inequality
% % \begin{equation}
% %     P\left( \left| \mathbf{\bar{p}}^k - \mathbb{E}[ \mathbf{\bar{p}}^k]  \right| \ge \varepsilon\right)  \le 2\exp(-2N\varepsilon^2).
% % \end{equation}
% % % We then have
% % % \begin{equation}
% % %     \mathbb{E}[\mathbf{\bar{p}}^k] = \frac{1}{N}\sum_{i=1}^N \mathbb{E}[\mathbf{p}_i^k]
% % % \end{equation} by the linearity of expectation.
% % By the definition of expectation. $\mathbb{E}[\mathbf{\bar{p}}]^k = \mathbb{E}[\mathbf{\bar{p}}^k]$, the above inequality means
% % \begin{equation}
% %     P\left( \left| \mathbf{\bar{p}}^k - \mathbb{E}[ \mathbf{\bar{p}}]^k  \right| \ge \varepsilon\right)  \le 2\exp(-2N\varepsilon^2).
% % \end{equation}
% % By Boole's inequality, this leads to
% % \begin{equation}
% % \label{eq:inftynorm_bound}
% % \begin{aligned}
% %     P\left(\left\| \mathbf{\bar{p}} - \mathbb{E}\left[ \mathbf{\bar{p}} \right] \right\|_\infty \ge \varepsilon\right) 
% %     & = P\left(\bigcup_k \left\{\left| \mathbf{\bar{p}}^k - \mathbb{E}[ \mathbf{\bar{p}}]^k \right| \ge \varepsilon \right\} \right) \\
% %     & \le \sum_k P\left( \left| \mathbf{\bar{p}}^k - \mathbb{E}[ \mathbf{\bar{p}}]^k \right| \ge \varepsilon \} \right) \\
% %     & \le 2K\exp(-2N\varepsilon^2)
% % \end{aligned}
% % \end{equation}

% For any $\mathbf{q} \in \mathbb{R}^K$, by the equivalence of $p$-norm we have $\|\mathbf{q}\| \le \|\mathbf{q}\|_1$. % \jingbo{do you want to use $\|\mathbf{q}\|_p$ here? Omitting $p$ is fine to me.} 
% Therefore,
% \begin{equation}
%   \left\{\mathbf{q} ~|~ \|\mathbf{q}\|  \ge \varepsilon \right\} \subseteq  \left\{\mathbf{q} ~|~ \|\mathbf{q}\|_1 \ge \varepsilon  \right\}.
% \end{equation}
% This implies, 
% \begin{equation}
%     \label{eq:p_norm_probability_inequality}
%     P\left(\left\| \mathbf{q} \right\| \ge \varepsilon\right)  \le P\left(\left\| \mathbf{q} \right\|_1 \ge \varepsilon\right) .
% \end{equation}

% Combine inequality (\ref{eq:classic_bound}) and (\ref{eq:p_norm_probability_inequality}) we then have
% \begin{equation}
%     P\left(\left\| \mathbf{\bar{p}} - \mathbb{E}\left[ \mathbf{\bar{p}} \right] \right\| \ge \varepsilon\right)  \le 2\exp \left(-\frac{N}{2K} \varepsilon^2 \right).
% \end{equation}



% % Let $\mathbf{p}^k$ denote the $k$-th coordinate of a vector $\mathbf{p}$. Let $\bar{\mathbf{y}} = N^{-1} \sum_{i=1}^N \mathbf{1}_{y_i}$. Since $\mathbf{1}_y^k \sim \mathbf{q}^k$, by Hoeffding's inequality we have
% % \begin{equation}
% %     P\left( | \bar{\mathbf{y}}^k - \mathbf{q}^k  | \ge \varepsilon\right)  \le 2\exp(-2N\varepsilon^2).
% % \end{equation}
% % Subsequently, by Boole's inequality we have
% % \begin{equation}
% % \begin{aligned}
% %     P\left(\left\| \bar{\mathbf{y}} - \mathbf{q} \right\|_\infty \ge \varepsilon\right) 
% %     & = P\left(\bigcup_k \left\{|\bar{\mathbf{y}}^k - \mathbf{q}^k| \ge \varepsilon \right\} \right) \\
% %     & \le \sum_k P\left( | \bar{\mathbf{y}}^k - \mathbf{q}^k  | \ge \varepsilon \} \right) \\
% %     & \le 2K\exp(-2N\varepsilon^2)
% % \end{aligned}
% % \end{equation}
% % % \jingbo{I have changed $N^{-1}$ to $1/N$ in the definition of $\bar{\mathbf{y}}$. probably do the same for $K^{-1}$. It's a bit odd to me with $^{-1}$} \chengyu{$1/N...$ would be confusing in in-line equation.}
% % By the equivalence of $p$-norm $K^{-1}\|\mathbf{q}\| \le \|\mathbf{q}\|_\infty$, we have
% % \begin{equation}
% %   \left\{\mathbf{q} | K^{-1} \|\mathbf{q}\|  \ge \varepsilon \right\} \subseteq  \left\{\mathbf{q} | \|\mathbf{q}\|_\infty \ge \varepsilon  \right\}.
% % \end{equation}
% % Therefore,
% % \begin{equation}
% %     P\left(\left\| \bar{\mathbf{y}} - \mathbf{q} \right\| \ge K \varepsilon\right)  \le 2K\exp(-2N\varepsilon^2).
% % \end{equation}

% \end{proof}

% % By a generalization of Hoeffding's inquality to category distribution (Lemma~\ref{lemma:sample-mean}), 
% Now we proceed to prove Lemma~\ref{lemma:sample-mean-relax}.

% First, since $x \in \mathcal{S}^r_j$, we have
% \begin{equation}
%     \|x - \bar{x}_j\| \le r,
% \end{equation}
% which implies $\forall x, x' \in \mathcal{S}^r_j$,
% \begin{equation}
%     \|x - x'\| \le 2r.
% \end{equation}
% Let $N_{\mathcal{S}} = |\mathcal{S}^r_j|$. By the locally Lipschitz continuity of $\mathbf{p}^*$ we can see that for any $x \in \mathcal{S}^r_j$,
% \begin{equation}
%     \left\|\mathbf{p}^*(x) - \frac{1}{N_{\mathcal{S}}} \sum_{x \in \mathcal{S}^r_j} \mathbf{p}^*(x)\right\| \le 2 \frac{N_{\mathcal{S}} - 1}{N_{\mathcal{S}}} L^* r \le 2 L^* r.
% \end{equation}
% The linearity of the expectation implies
% \begin{equation}
%     \mathbb{E}[\mathbf{\bar{y}}] = {N_{\mathcal{S}}}^{-1} \sum_{x \in \mathcal{S}^r_j} \mathbb{E}[\mathbf{1}_{y(x)}] = {N_{\mathcal{S}}}^{-1} \sum_{x \in \mathcal{S}^r_j} \mathbf{p}^*(x).
% \end{equation}
% Therefore
% \begin{equation}
%     \left\|\mathbf{p}^*(x) - \mathbb{E}[\mathbf{\bar{y}}] \right\| \le 2 L^* r.
% \end{equation}

% By the triangle inequality we have
% \begin{equation}
%     \|\mathbf{p}^*(x) - \bar{\mathbf{y}} \| \le \|\mathbf{p}^*(x) - \mathbb{E}[\bar{\mathbf{y}}] \| + \|\mathbb{E}[\bar{\mathbf{y}}] - \bar{\mathbf{y}} \|.
% \end{equation}
% This implies
% \begin{equation}
%      P\left( \|\mathbf{p}^*(x) - \bar{\mathbf{y}} \| \ge \varepsilon\right) \le P\left( \| \bar{\mathbf{y}} - \mathbb{E}[\bar{\mathbf{y}}] \| \ge \tilde{\varepsilon}\right),
% \end{equation}
% where $\tilde{\varepsilon} = \varepsilon - 2 L^* r$.
% Apply Lemma~\ref{lemma:sample-mean} we then have
% \begin{equation}
%      P\left( \|\mathbf{p}^*(x_i) - \bar{\mathbf{y}} \| \ge \tilde{\varepsilon}\right) \le 2\exp\left(-\frac{N_{\mathcal{S}}}{2K^2}\tilde{\varepsilon}^2\right),
% \end{equation}

% \end{proof}





% \subsection{Proof of Lemma~\ref{lemma:vector-minimization}}
% \begin{proof}

% We rephrase the problem~(\ref{eq:minimum-partition}) as 

% \begin{equation}
% \label{eq:vector-minimization2}
% \begin{aligned}
%     \min_{\{\mathbf{p}_i\}_{i=1}^N} & - \frac{1}{N} \sum_{i} \mathbf{1}_{y_i} \cdot \log \mathbf{p}_i \\
%     s.t.~~& \|\mathbf{p}_i - \mathbf{p}\| \le \varepsilon, ~\sum_k \mathbf{p}_i^k = 1, ~\sum_k \mathbf{p}^k = 1, \mathbf{p}^k_i \ge 0, \mathbf{p}^k \ge 0. \\
% \end{aligned}
% \end{equation}
% % \jingbo{the second summation in s.t. should loop over $k$ too?}

% % \chengyu{What if $\mathbf{p}^{y_i} + \varepsilon > 1$?}
% % \chengyu{If there exists one like this and it is in the feasible set. Then means one entry of $p$ is close to $1$. If in this case $p$ can still be the minimizer, then means the sample mean has to be close to one hot, which means true label distribution is close to one-hot. Therefore this is a trivial case.}
% % \jingbo{can we assume $\varepsilon$ is very small? Then, empirically it will be always feasible, at least in the floating number computation in computers?}
% % \jingbo{also, I think you missed the constraint that all $\mathbf{p}$ and $\mathbf{p}_i$ values must be non-negative?}
% % \chengyu{Since we have $\log$, this is implicit. And even if we have this constraint in KKT condition it only contributes to a constant. Therefore the result is the same.}
% % \jingbo{Since we are mainly to derive a bound, we can relax some of the constraints? Relaxing the constraint will only make the optimal value smaller. The bound should still hold.} \chengyu{we cannot relax, we are deriving the property of minimizer, not the minimum.}
% \smallsection{Case I}
% % \chengyu{Add positive constraint}
% We first discuss the case when $\mathbf{p}^k + \varepsilon < 1$ for all $k$. 
% First, we observe that for any $\mathbf{p}$, the minimum of the above problem is achieved only if $\mathbf{p}_i^{y_i} = \mathbf{p}^{y_i} + \varepsilon$. Because by contradiction, if $\mathbf{p}_i^{y_i} < \mathbf{p}^{y_i} + \varepsilon$, we will have $-\log \mathbf{p}_i^{y_i} > -\log(\mathbf{p}^{y_i} + \varepsilon) $, and $\mathbf{p}^{y_i} + \varepsilon$ belongs to the feasible set, which means $\mathbf{p}_i^{y_i}$ does not attain the minimum.

% The above problem can then be rephrased as
% \begin{equation}
% \begin{aligned}
%     \min_{\mathbf{p}} - \frac{1}{N} \sum_{i} \log( {\mathbf{p}}^{y_i} + \varepsilon),~~ s.t.~~\sum_k \mathbf{p}^k = 1, \mathbf{p}^k \ge 0,
% \end{aligned}
% \end{equation}
% where we have neglected the condition associated with $\mathbf{p}_i^{k\ne y_i}$, since they do not contribute to the objective, they can be chosen arbitrarily as long as the constraints are sufficed, and clearly the constraints are underdetermined.

% Let $N_k = \sum_i 1(y_i = k)$, we have $\sum_i \log (\mathbf{p}^{y_i} + \varepsilon) = \sum_k N_k \log (\mathbf{p}^k + \varepsilon)$. Therefore the above problem is equivalent to
% \begin{equation}
% \begin{aligned}
%     \label{eq:convex-minimization}
%     \min_{\mathbf{p}}- \sum_k \mathbf{\bar{y}}^k \log (\mathbf{p}^k + \varepsilon),~~ s.t.~~\sum_k \mathbf{p}^k = 1, \mathbf{p}^k \ge 0,
% \end{aligned}
% \end{equation}
% where $\mathbf{\bar{y}} \equiv [N_1 / N, \cdots, N_k / N]^T $ is equal to the sample mean $N^{-1}\sum_i \mathbf{1}_{y_i}$. 

% To solve the strongly convex minimization problem (\ref{eq:convex-minimization}) it is easy to employ KKT conditions to show that  
% $$ \mathbf{p} = \mathbf{\bar{y}} (1 + K\varepsilon) - \varepsilon. 
% $$

% % \vspace{0.1em}
% \smallsection{Case II} We now discuss the case when $\mathbf{\hat{p}}$ is the minimizer of (\ref{eq:vector-minimization2}) and there exists $k'$ such that $\mathbf{\hat{p}}^{k'} + \varepsilon \ge 1$. And $\mathbf{\hat{p}}\ne \mathbf{p}^*$, where $\mathbf{p}^* = \mathbf{\bar{y}}(1+K\varepsilon) - \varepsilon$ is the form of the minimizer in the previous case.

% Considering a non-trivial case $\mathbf{p^*}^{k'} < 1 - \varepsilon$. Otherwise the true label distribution is already close to the one-hot labeling, which is the minimizer of the empirical risk. Therefore by $\sum_{k\ne k'} {\mathbf{p}^*}^{k} > \varepsilon$ we have the condition
% \begin{equation}
%     \sum_{k\ne k'}\mathbf{\bar{y}}^k >  \frac{K\varepsilon}{1 + K\varepsilon}
% \end{equation}


% Now considering the minimization objective $R(p) = - {N}^{-1} \sum_i \mathbf{1}_{y_i} \cdot \log \mathbf{p}_i$. For all $i$ with $y_i = k'$, we must have $\mathbf{p}_i^{y_i} = 1$, otherwise the optimal cannot be attained by contradiction. Then the minimization problem can be rephrased as
% \begin{equation}
%     \min \sum_{k\ne k'} \mathbf{\bar{y}}^k \log (\mathbf{\hat{p}} + \varepsilon), ~s.t. \sum_{k'\ne k} \mathbf{\hat{p}}^{k} \ge \varepsilon, \mathbf{\hat{p}}^{k} \ge 0,
% \end{equation}
% where the first constraint is imposed by $\mathbf{\hat{p}}^{k'} \ge 1 - \varepsilon$.


% Employ KKT conditions similarly we can have $\mathbf{\hat{p}}^k = \mathbf{\bar{y}}^k/\lambda - \varepsilon$ where $\lambda$ is a constant. By checking the constraint we can derive $\lambda \ge \sum_k \mathbf{\bar{y}}^k / (K\varepsilon)$.

% However, the minimization objective 
% $$
% \min_{\lambda} - \sum_{k\ne k'} \mathbf{\bar{y}}^k \log \frac{\mathbf{\bar{y}}^k}{\lambda},
% $$
% requires $\lambda$ to be minimized. Therefore $\lambda = \sum_{k\ne k'} \mathbf{\bar{y}}^k / (K\varepsilon)$, which implies
% \begin{equation}
% \mathbf{\hat{p}}^k = K\varepsilon \frac{\mathbf{\bar{y}}^k}{\sum_{k\ne k'} \mathbf{\bar{y}}^k} - \varepsilon.
% \end{equation}

% Now since $\mathbf{\hat{p}} = \arg\min_p R(p)$ and $\mathbf{\hat{p}} \ne \mathbf{p}^*$, we must have $R(\mathbf{\hat{p}}) < R(\mathbf{p}^*)$. This means
% \begin{equation}
%  - \sum_{k\ne k'} \mathbf{\bar{y}}^k \log \frac{K\varepsilon \mathbf{\bar{y}}^k}{\sum_{k\ne k'} \mathbf{\bar{y}}^k} < - \sum_{k\ne k'} \mathbf{\bar{y}}^k \log [\mathbf{\bar{y}}^k(1+K\varepsilon)],
% \end{equation}
% which is reduced to
% \begin{equation}
% \sum_{k\ne k'}\mathbf{\bar{y}}^{k} < \frac{K\varepsilon}{1+K\varepsilon}
% \end{equation}
% But this is contradict to our assumption.
% \end{proof}
