# Supplementary material for: Toward Student-Oriented Teacher Network Training For Knowledge Distillation
Source: arXiv:2206.06661 source file (2024-05-09)
Supplement: Supplementary file 3 [file 41_proof_of_theorem_41.tex]

% -------------------------------------
\section{Proof of Theorem~\ref{theorem:error}}
\label{sect:proof_41}
% \smallsection{Step I: Partition the training inputs}
\smallsection{Step I: Bound the difference between the true label distribution and the sample mean}
% \chengyu{Convert to pac}
First we note that the set of all training inputs can be grouped into several subsets such that the inputs in each subset possess similar true label distribution. 

More formally, 
Let $\mathcal{C}_r^* = \{\bar{x}_j\}_{j=1}^{\sigma_r}$ be an $r$-external covering of $\mathcal{S}$ with minimum cardinality, namely
\begin{equation}
    \label{eq:covering}
    \mathcal{S} \subseteq \bigcup_{x \in \mathcal{C}_r^*} \{x' ~|~ \|x ' - x\| \le r \},
\end{equation}
where we refer $\bar{x}_j$ as the $r$-covering center, and $N_r$ is the $r$-covering number.

Let $\{\mathcal{S}^r_j\}_{j=1}^{\sigma_r}$ be any disjoint partition of $\mathcal{S}$ such that $\mathcal{S}_j^r \subseteq \{x' | \|x ' - \bar{x}_j\| \le r \}$. 
We show that $\mathcal{{S}}_j^r$ attains a property that the true label distribution $\bm{p}^*(x)$ of any input $x$ in this subset will not be too far from the sample mean of one-hot labels $\bm{\bar{y}}_j = {|\mathcal{{S}}_j^r|}^{-1} \sum_{x\in \mathcal{{S}}_j^r} \mathbf{1}_{y}$ in this subset. Namely given any $\varepsilon > 0$, we have
% , as shown by the following lemma.
% \begin{lemma}
% Let $\mathcal{{S}}(r)=\{x_i\}_{i=1}^{N_{\mathcal{{S}}}}$ be a collection of inputs constructed above and $N_{\mathcal{{S}}} \equiv |\mathcal{{S}}(r)|$. Let $\bar{\bm{y}} \equiv {N_{\mathcal{{S}}}}^{-1} \sum_i \mathbf{1}_{y^i}$. Then for any $i=1,\cdots, N_{\mathcal{{S}}}$,
% \begin{equation}
%      P\left( \|\bm{p}^*(x_i) - \bar{\bm{y}} \| \ge \varepsilon\right) \le 2K\exp\left(-2\frac{N}{K^2}{\varepsilon}^2\right),
% \end{equation}
% where ${\varepsilon} = \varepsilon - L^* r$.
% \end{lemma}
\begin{equation}
     \label{lemma:sample-mean-relax}
     P\left( \|\bm{p}^*(x) - \bar{\bm{y}}_j \| \ge \varepsilon\right) \le 2\exp\left(-\frac{|\mathcal{S}_j^r|}{2K}\tilde{\varepsilon}^2\right),
\end{equation}
where $\tilde{\varepsilon} = \max(\varepsilon - 2 rL_p, 0)$.

To prove this property we first present two lemmas. 
\begin{lemma}[Lipschitz constraint of the true label distribution]
\label{lemma:Lipschitz-true-distribution}
Let $\mathcal{S}_j^r$ be a subset constructed above and $\bm{\bar{y}}_j = {|\mathcal{{S}}_j^r|}^{-1} \sum_{x\in \mathcal{{S}}_j^r} \mathbf{1}_{y}$. Then for any $x \in \mathcal{S}_j^r$ we have,
\begin{equation}
    \left\|\bm{p}^*(x) - \mathbb{E}[\bm{\bar{y}}_j] \right\| \le 2 rL_p.
\end{equation}
\end{lemma}
\begin{proof}
% \chengyu{Show the proof here so we don't have to introduce local Lipschitz somewhere}
% See detailed proof in Appendix~\ref{section:all-proof}.
First, since $x \in \mathcal{S}^r_j$, we have $\|x - \bar{x}_j\| \le r $, which implies $\|\bm{p}^*(x) - \bm{p}^*(\bar{x}_j)\| \le rL_p$ by the locally Lipschitz continuity of $\bm{p}^*$. Then for any $x, x' \in \mathcal{S}^r_j$, we will have $\|\bm{p}^*(x) - \bm{p}^*(x')\| \le 2rL_p$ by the triangle inequality. Let $N_{\mathcal{S}} = |\mathcal{S}^r_j|$. Therefore,
\begin{equation}
    \left\|\bm{p}^*(x) - \frac{1}{N_{\mathcal{S}}} \sum_{x \in \mathcal{S}^r_j} \bm{p}^*(x)\right\| \le 2 \frac{N_{\mathcal{S}} - 1}{N_{\mathcal{S}}} rL_p \le 2 rL_p.
\end{equation}
Further, the linearity of the expectation implies
\begin{equation}
    \mathbb{E}[\bm{\bar{y}}] = {N_{\mathcal{S}}}^{-1} \sum_{x \in \mathcal{S}^r_j} \mathbb{E}[\mathbf{1}_{y(x)}] = {N_{\mathcal{S}}}^{-1} \sum_{x \in \mathcal{S}^r_j} \bm{p}^*(x).
\end{equation}
Therefore $ \left\|\bm{p}^*(x) - \mathbb{E}[\bm{\bar{y}}_j] \right\| \le 2 rL_p$.
\end{proof}


\begin{lemma}[Concentration inequality of the sample mean]
\label{lemma:sample-mean}
% Let $\mathbf{1}_y$ be the one-hot label of an input $x$. 
Let $\mathcal{S}$ be a set of $x$ with cardinality $N$.
Let $\bm{\bar{y}} = N^{-1} \sum_{x\in \mathcal{S}} \mathbf{1}_y$ be the sample mean.
Then for any $p$-norm $\|\cdot\|$ and any $\varepsilon > 0$,  we have 
% \chengyu{or maybe $\tilde{\varepsilon} > 0$?? otherwise negative. Or $\max(\tilde{\varepsilon}, 0)$. When $\tilde{\varepsilon} = 0$ the bound is trivial, namely a norm of course will be larger than $0$.}
\begin{equation}
    \label{eq:concentration-sample-mean}
    P\left(\left\| \bm{\bar{y}} - \mathbb{E}\left[ \bm{\bar{y}} \right] \right\| \ge \varepsilon\right)  \le 2\exp\left(-\frac{N}{2K}\varepsilon^2\right).
\end{equation}
\end{lemma}

\begin{proof}

% Concentration inequality to the category distribution

% by the linearity of expectation and concentration inequality to a category distribution.
% % See detailed proof in Appendix~\ref{section:all-proof}.

% Note that a category distribution can be viewed as a special case of a multinomial distribution. 
Note that $\bm{\bar{y}}$ obeys a multinomial distribution, \emph{i.e.} $\bm{\bar{y}} \sim N^{-1} multinomial(N, \mathbb{E}[\bm{\bar{y}}])$.
We utilize the classic results on the concentration properties of multinomial distribution based on $\ell_1$ norm~\cite{Weissman2003InequalitiesFT, Qian2020ConcentrationIF}, namely
\begin{equation}
\label{eq:classic_bound}
P(\left\| \bm{\bar{y}} - \mathbb{E}\left[ \bm{\bar{y}} \right] \right\|_1 \ge \varepsilon) \le 2\exp\left({-\frac{N}{2 K}\varepsilon^2}\right)
\end{equation}

Further, for any $\bm{q} \in \mathbb{R}^K$, by the equivalence of $p$-norm we have $\|\bm{q}\| \le \|\bm{q}\|_1$. % \jingbo{do you want to use $\|\bm{q}\|_p$ here? Omitting $p$ is fine to me.} 
Therefore,
\begin{equation}
  \left\{\bm{q} ~|~ \|\bm{q}\|  \ge \varepsilon \right\} \subseteq  \left\{\bm{q} ~|~ \|\bm{q}\|_1 \ge \varepsilon  \right\},
\end{equation}
which implies, 
\begin{equation}
    \label{eq:p_norm_probability_inequality}
    P\left(\left\| \bm{q} \right\| \ge \varepsilon\right)  \le P\left(\left\| \bm{q} \right\|_1 \ge \varepsilon\right) .
\end{equation}

Combine inequality (\ref{eq:classic_bound}) and (\ref{eq:p_norm_probability_inequality}) we then have (\ref{eq:concentration-sample-mean}).
% \begin{equation}
%     P\left(\left\| \bm{\bar{y}} - \mathbb{E}\left[ \bm{\bar{y}} \right] \right\| \ge \varepsilon\right)  \le 2\exp \left(-\frac{N}{2K} \varepsilon^2 \right).
% \end{equation}
\end{proof}


One can see that Lemma~\ref{lemma:Lipschitz-true-distribution} bounds the difference between true label distribution of individual inputs and the mean true label distribution, while Lemma~\ref{lemma:sample-mean} bounds the difference between the sample mean and the mean true label distribution. Therefore the difference between the true label distribution and the sample mean is also bounded, since by the triangle inequality we have
\begin{equation}
    \|\bm{p}^*(x) - \bar{\bm{y}} \| \le \|\bm{p}^*(x) - \mathbb{E}[\bar{\bm{y}}] \| + \| \bar{\bm{y}} - \mathbb{E}[\bar{\bm{y}}] \|.
\end{equation}
This implies
\begin{equation}
     P\left( \|\bm{p}^*(x) - \bar{\bm{y}} \| \ge \varepsilon\right) \le P\left( \| \bar{\bm{y}} - \mathbb{E}[\bar{\bm{y}}] \| \ge \tilde{\varepsilon}\right),
\end{equation}
where $\tilde{\varepsilon} = \max(\varepsilon - 2 rL_p, 0)$.
Apply Lemma~\ref{lemma:sample-mean} we then have (\ref{lemma:sample-mean-relax}).
% \begin{equation}
%      P\left( \|\bm{p}^*(x_i) - \bar{\bm{y}} \| \ge \tilde{\varepsilon}\right) \le 2\exp\left(-\frac{N_{\mathcal{S}}}{2K^2}\tilde{\varepsilon}^2\right),
% \end{equation}
% which arrives at 


% \begin{lemma}
% \label{lemma:sample-mean-relax}
% Let $\mathcal{S}^r_j$ be a collection of inputs constructed above. Let $\bar{\bm{y}}_j = {|\mathcal{S}_j^r|}^{-1} \sum_{x\in \mathcal{S}_j^r} \mathbf{1}_{y}$, where $y$ is the label of $x$. Then for any $x \in \mathcal{S}^r_j$, for any $p$-norm $\|\cdot\|$ and any $\varepsilon > 0$,
% \begin{equation}
%      P\left( \|\bm{p}^*(x) - \bar{\bm{y}}_j \| \ge \varepsilon\right) \le 2\exp\left(-\frac{|\mathcal{S}_j^r|}{2K}\tilde{\varepsilon}^2\right),
% \end{equation}
% where $\tilde{\varepsilon} = \varepsilon - 2 L^* r$.
% \end{lemma}

% \begin{proof}
%  We first bound the difference between the sample mean and the mean true label distribution by the linearity of expectation and Hoeffding's inequality generalized to a category distribution. Then utilize local Lipschitz continuity of the true label distribution to bound the difference between true label distribution of individual inputs and the mean true label distribution. Therefore the difference between the true label distribution and the sample mean is also bounded. See detailed proof in Appendix~\ref{section:all-proof}.

% \end{proof}


\vspace{1em}
\smallsection{Step II: Bound the difference between the prediction given by the empirical risk minimizer and the sample mean}
% \smallsection{Step II: Find the minimizer of the empirical risk with Lipschitz constraint} 
Here we show that given the locally Lipschitz constraint established in each disjoint partition we constructed above, the prediction given by the empirical risk minimizer will be close to the sample mean. As an example, we focus on the negative log-likelihood loss, namely $\ell(\bm{f}(x), y) = - \mathbf{1}_y \cdot \log \bm{f} (x) $. Other loss functions that are subject to the proper scoring rule can be investigated in a similar manner.

% First, we regroup the sum in (\ref{eq:lip-minimization}) based on the partition constructed above, namely
% \begin{equation}
%     \hat{R}(\bm{f}, \mathcal{S}) = \frac{1}{N_{\bm{q}} M} \sum_{\{\bm{q}\}}\sum_{m=1}^M \hat{R} (\bm{f}, \mathcal{S}_m(\bm{q})),
% \end{equation}
% where $\hat{R} (\bm{f}, \mathcal{S}_m(\bm{q})) = -{|\mathcal{S}_m(\bm{q})|}^{-1} \sum_{x\in \mathcal{S}_m(\bm{q})} \mathbf{1}_y \cdot \log \bm{f}(x)$ is the empirical risk in each partition.  The goal is to find $\bm{f}$ that minimizes  $\hat{R} (\bm{f}, \mathcal{S}_m(\bm{q}))$ in each partition given the local Lipschitz constraint, namely
% \begin{equation}
% \label{eq:minimum-partition}
% \begin{aligned}
% & \min \hat{R} (\bm{f}, \mathcal{S}_m(\bm{q}))\\
% &~s.t.~~ \|\bm{f}(x) - \bm{f}(\bar{x}_m)\| \le Lr, ~\forall~x \in \mathcal{S}_m(\bm{q}).
% \end{aligned}
% \end{equation}

First, we regroup the sum in (\ref{eq:empirical-risk}) based on the partition constructed above, namely
% \lucas{small bug fixed.}
\begin{equation}
    \hat{R}(\bm{f}, \mathcal{S}) = \frac{1}{N_r}\sum_{j=1}^{N_r}  |\mathcal{S}_j^r| \cdot \hat{R}(\bm{f}, \mathcal{S}_j^r),
\end{equation}
where $\hat{R} (\bm{f}, \mathcal{S}_j^r) = -{|\mathcal{S}_j^r|}^{-1} \sum_{i=1}^{|\mathcal{S}_j^r|} \mathbf{1}_{y_i} \cdot \log \bm{f}(x_i)$ is the empirical risk in each partition. Since we are only concerned with the existence of a desired minimizer of the empirical risk, we assume that $\bm{f}$ is able to achieve any labeling of the training inputs that suffices the local Lipschitz constraint. 
% \chengyu{This is the only problem left, there are additional constraints imposed by those perimeter inputs that are close to other centers. In this case considering the Lipschitz continuity of true distribution at the scale of $2r$, and show the additional constraint would not affect the miniizer a lot?} 
Thus the empirical risk minimization is equivalent to the minimization of the empirical risk in each partition.
The problem can thus be defined as, for each $j \in \{1, \cdots, N_r\}$,
% The goal is that for each $j$, find $\bm{p}_i = \bm{f}(x_i)$ and $\mathbf{\bar{p}} = \bm{f}(\bar{x}_j)$ for each $i=1,\cdots, |\mathcal{S}_j(r)|$ that minimizes $\hat{R} (\bm{f}, \mathcal{S}_j(r))$, given the constraint $\|\bm{p}_i - \bm{p}\| \le Lr $, which is imposed by the local Lipschitz continuity of the function $\bm{f}$.
% \chengyu{The bound is due to all examples are within $r$ from $\bar{x}$}
% Now define the minimization problem as 
\begin{equation}
\label{eq:minimum-partition}
\begin{aligned}
& \min_{\bm{f}} \hat{R} (\bm{f}, \mathcal{S}_j^r)\\
& s.t.~~ \|\bm{f}(x) - \bm{f}(\bar{x}_j)\| \le rL_f, 
% ~\forall~i=1,\cdots, |\mathcal{S}_j(r)|.
~\forall~x \in \mathcal{S}_j^r,
\end{aligned}
\end{equation}
where the constraint is imposed by the locally-Lipschitz continuity of $\bm{f}$. By the following lemma, we show that the minimizer of such problem is achieved only if $\bm{f}(\bar{x}_j)$ is close to the sample mean.


% Under an ideal circumstance $L = 0$, which means $\bm{f}(x) = \bm{f}(\bar{x}_m)$ for all $x$, the minimum of (\ref{eq:minimum-partition}) must be attained when $\bm{f}(x) = \bar{\bm{y}}_m$, as it is easy to see that by Gibbs inequality
% \begin{equation}
%     - \sum_{x\in \mathcal{S}_m(\bm{q})} \mathbf{1}_y \cdot \log \bm{f}(\bar{x}_m)  \ge - {|\mathcal{S}_m(\bm{q})|} \sum_{x\in \mathcal{S}_m(\bm{q})} \mathbf{1}_y \cdot \log \bar{\bm{y}}_m,
% \end{equation}
% and the equality is achieved if and only if $\bm{f}(\bar{x}_m) = \bar{\bm{y}}_m$. We show by Lemma~\ref{lemma:vector-minimization} that with a relaxed condition $L > 0$, the optimal predictions are not too far from $\bar{y}_m$.

\begin{lemma}
\label{lemma:vector-minimization}
% \chengyu{All argmax values will try to be as close to $1$ as possible. Therefore it has to be $p_y + \varepsilon$? Otherwise can always move closer given convexity by contradiction. Then we can group the sum of all examples have the same one-hot label.}
Let $\bar{\bm{y}} ={|\mathcal{S}_j^r|}^{-1} \sum_{x \in \mathcal{S}_j^r} \mathbf{1}_{y}$.  The minimum of the problem (\ref{eq:minimum-partition}) is achieved if and only if $\bm{f}(\bar{x}_j) = \mathbf{\bar{y}_j}(1 + rKL_f) - rL_f$.

% Let $\bm{p}_i, \bm{p} \in [0, 1]^K$. The minimum of the problem 
% \begin{equation}
% \begin{aligned}
%     \min_{\{\bm{p}_i\}_{i=1}^N} & - \frac{1}{N} \sum_{i} \mathbf{1}_{y_i} \cdot \log \bm{p}_i \\
%     % \cdot \log (\bm{p} + \varepsilon), \\
%     s.t.~~& \|\bm{p}_i - \bm{p}\| \le \varepsilon, ~\sum_j \bm{p}_i^j = 1, ~\sum_j \bm{p}^j = 1 \\
% \end{aligned}
% \end{equation}
% is attained only if
% \begin{equation}
% \begin{aligned}
%     & \bm{p} = \bm{\bar{y}}(1 + K\varepsilon) - \varepsilon,\\
%     % & (\bm{p}_i^*)^{y_i} = (\bm{p}^*)^{y_i} + \varepsilon, \\
%     % & (\bm{p}_i^*)^{k\ne y_i} = (\bm{p}^*)^{k\ne y_i} - \delta_i^k, 
% \end{aligned}
% \end{equation}
% where $\bar{\bm{y}} = N^{-1} \sum_i \mathbf{1}_{y_i}$.
% % and $\delta_i^k \ge 0$ can be chosen arbitrarily as long as it suffices the constraints $\|\bm{p}^*_i - \bm{p}^*\| \le \varepsilon$ and $\sum_j (\bm{p}_i^*)^j = 1$.
\end{lemma}

\begin{proof}
We note that since the loss function we choose is strongly convex, to minimize the empirical risk, the prediction of any input $x$ must be as close to the one-hot labeling as possible. Therefore the problem (\ref{eq:minimum-partition}) can be formulated into a vector minimization where we can employ Karush–Kuhn–Tucker (KKT) theorem to find the necessary conditions of the minimizer. 
% See detailed proof in Appendix~\ref{section:all-proof}.
% \end{proof}

% \subsection{Proof of Lemma~\ref{lemma:vector-minimization}}
% \begin{proof}
We rephrase the problem~(\ref{eq:minimum-partition}) as
\begin{equation}
\label{eq:vector-minimization2}
\begin{aligned}
    \min_{\{\bm{p}_i\}_{i=1}^N} & - \frac{1}{N} \sum_{i} \mathbf{1}_{y_i} \cdot \log \bm{p}_i \\
    s.t.~~& \|\bm{p}_i - \bm{p}\| \le \varepsilon, ~\sum_k \bm{p}_i^k = 1, ~\sum_k \bm{p}^k = 1,\\
    & \bm{p}^k_i \ge 0, \bm{p}^k \ge 0. \\
\end{aligned}
\end{equation}
where $\bm{p}^k_i$ is the $k$-th dimension of $\bm{f}(x_i)$ and $\bm{p}^k$ is the $k$-th dimension of $\bm{f}(\bar{x}_j)$. 
% \lucas{double check here.}  

\smallsection{Case I}
We first discuss the case when $\bm{p}^k + \varepsilon < 1$ for all $k$. 
First, we observe that for any $\bm{p}$, the minimum of the above problem is achieved only if $\bm{p}_i^{y_i} = \bm{p}^{y_i} + \varepsilon$. Because by contradiction, if $\bm{p}_i^{y_i} < \bm{p}^{y_i} + \varepsilon$, we will have $-\log \bm{p}_i^{y_i} > -\log(\bm{p}^{y_i} + \varepsilon) $, and $\bm{p}^{y_i} + \varepsilon$ belongs to the feasible set, which means $\bm{p}_i^{y_i}$ does not attain the minimum.

The above problem can then be rephrased as
\begin{equation}
\begin{aligned}
    \min_{\bm{p}}& - \frac{1}{N} \sum_{i} \log( {\bm{p}}^{y_i} + \varepsilon)\\
    s.t.~~&\sum_k \bm{p}^k = 1, \bm{p}^k \ge 0,
\end{aligned}
\end{equation}
where we have neglected the condition associated with $\bm{p}_i^{k\ne y_i}$, since they do not contribute to the objective, they can be chosen arbitrarily as long as the constraints are sufficed, and clearly the constraints are underdetermined.

Let $N_k = \sum_i 1(y_i = k)$, we have $\sum_i \log (\bm{p}^{y_i} + \varepsilon) = \sum_k N_k \log (\bm{p}^k + \varepsilon)$. Therefore the above problem is equivalent to
\begin{equation}
\begin{aligned}
    \label{eq:convex-minimization}
    \min_{\bm{p}}- \sum_k \bm{\bar{y}}^k \log (\bm{p}^k + \varepsilon),~~ s.t.~~\sum_k \bm{p}^k = 1, \bm{p}^k \ge 0,
\end{aligned}
\end{equation}
where $\bm{\bar{y}} \equiv [N_1 / N, \cdots, N_k / N]^T $ is equal to the sample mean $N^{-1}\sum_i \mathbf{1}_{y_i}$. 

To solve the strongly convex minimization problem (\ref{eq:convex-minimization}) it is easy to employ KKT conditions to show that  
$$ \bm{p} = \bm{\bar{y}} (1 + K\varepsilon) - \varepsilon. 
$$

% \vspace{0.1em}
\smallsection{Case II} We now discuss the case when $\bm{\hat{p}}$ is the minimizer of (\ref{eq:vector-minimization2}) and there exists $k'$ such that $\bm{\hat{p}}^{k'} + \varepsilon \ge 1$. And $\bm{\hat{p}}\ne \bm{p}^*$, where $\bm{p}^* = \bm{\bar{y}}(1+K\varepsilon) - \varepsilon$ is the form of the minimizer in the previous case.

Considering a non-trivial case $\mathbf{p^*}^{k'} < 1 - \varepsilon$. Otherwise the true label distribution is already close to the one-hot labeling, which is the minimizer of the empirical risk. Therefore by $\sum_{k\ne k'} {\bm{p}^*}^{k} > \varepsilon$ we have the condition
\begin{equation}
    \sum_{k\ne k'}\bm{\bar{y}}^k >  \frac{K\varepsilon}{1 + K\varepsilon}
\end{equation}


Now considering the minimization objective $R(p) = - {N}^{-1} \sum_i \mathbf{1}_{y_i} \cdot \log \bm{p}_i$. For all $i$ with $y_i = k'$, we must have $\bm{p}_i^{y_i} = 1$, otherwise the optimal cannot be attained by contradiction. Then the minimization problem can be rephrased as
\begin{equation}
    \min \sum_{k\ne k'} \bm{\bar{y}}^k \log (\bm{\hat{p}} + \varepsilon), ~s.t. \sum_{k'\ne k} \bm{\hat{p}}^{k} \ge \varepsilon, \bm{\hat{p}}^{k} \ge 0,
\end{equation}
where the first constraint is imposed by $\bm{\hat{p}}^{k'} \ge 1 - \varepsilon$.


Employ KKT conditions similarly, we can have $\bm{\hat{p}}^k = \bm{\bar{y}}^k/\lambda - \varepsilon$ where $\lambda$ is a constant. By checking the constraint we can derive $\lambda \ge \sum_k \bm{\bar{y}}^k / (K\varepsilon)$.

However, the minimization objective 
$$
\min_{\lambda} - \sum_{k\ne k'} \bm{\bar{y}}^k \log \frac{\bm{\bar{y}}^k}{\lambda},
$$
requires $\lambda$ to be minimized. Therefore $\lambda = \sum_{k\ne k'} \bm{\bar{y}}^k / (K\varepsilon)$, which implies
\begin{equation}
\bm{\hat{p}}^k = K\varepsilon \frac{\bm{\bar{y}}^k}{\sum_{k\ne k'} \bm{\bar{y}}^k} - \varepsilon.
\end{equation}

Now since $\bm{\hat{p}} = \arg\min_p R(p)$ and $\bm{\hat{p}} \ne \bm{p}^*$, we must have $R(\bm{\hat{p}}) < R(\bm{p}^*)$. This means
\begin{equation}
 - \sum_{k\ne k'} \bm{\bar{y}}^k \log \frac{K\varepsilon \bm{\bar{y}}^k}{\sum_{k\ne k'} \bm{\bar{y}}^k} < - \sum_{k\ne k'} \bm{\bar{y}}^k \log [\bm{\bar{y}}^k(1+K\varepsilon)],
\end{equation}
which is reduced to
\begin{equation}
\sum_{k\ne k'}\bm{\bar{y}}^{k} < \frac{K\varepsilon}{1+K\varepsilon}
\end{equation}
But this is contradict to our assumption.
\end{proof}


% \smallsection{Step III: Bound the error between the minimizer's prediction and the sample mean}
We are now be able to bound the difference between the predictions of the training inputs produced by the empirical risk minimizer and the sample mean in each $\mathcal{S}_j^r$. To see that we have for each $x \in \mathcal{S}_j^r$. % This is straightforward to show as for all training inputs in each partition $x \in \mathcal{S}_j(r)$, 
\begin{equation}
\begin{aligned}
    \|\bm{f}(x) - \bm{\bar{y}}_j \| 
    & \le \|\bm{f}(x) - \bm{f}(\bar{x}_j) \| + \|\bm{f}(\bar{x}_j) - \bm{\bar{y}}_j \|  \\
    & \le rL_f ( 1 + K\|\bm{\bar{y}}_j -  K^{-1}\mathbf{1}\|)\\
    & \le rL_f ( 1 + K\|\mathbf{1}_{(\cdot)} - K^{-1}\mathbf{1}\|).\\
\end{aligned}
\end{equation}
% By Lemma~\ref{lemma:sample-mean-relax} we then have for any $x \in \mathcal{S}_j^r$, 
By Equation~(\ref{lemma:sample-mean-relax}) we then have for any $x \in \mathcal{S}_j^r$, 
\begin{equation}
    \label{eq:final-bound-each-partition}
    P\left(\|\bm{f}(x) - \bm{p}^*(x)\| \ge \varepsilon\right)  \le 2\exp\left(-\frac{|\mathcal{S}_j^r|}{2K}{\tilde{\varepsilon}}^2\right),
\end{equation}
which means the difference between the predictions and the true label distribution is also bounded. Here $\tilde{\varepsilon} = \max(\varepsilon - rL_f ( 1 + K\|\mathbf{1}_{(\cdot)} - K^{-1}\mathbf{1}\|) - 2 rL_p, 0)$.




\smallsection{Step III: Show the disjoint partition is non-trivial}
In (\ref{eq:final-bound-each-partition}), we have managed to bound the difference between the predictions yielded by an empirical risk minimizer and the true label distribution based on the cardinality of the subset $|\mathcal{S}_j^r|$, namely the number of inputs in $j$-partition. However $|\mathcal{S}_j^r|$ is critical to the bound here as if $|\mathcal{S}_j^r| = 1$, then (\ref{eq:final-bound-each-partition}) becomes a trivial bound. Here we show $|\mathcal{S}_j^r|$ is non-negligible based on simple combinatorics.

\begin{lemma}
\label{lemma:bound-partition}
Let $\{\mathcal{S}^r_j\}_{j=1}^{N_r}$ be a disjoint partition of the entire training set $\mathcal{S}$. Denote $\mathcal{S}^r(x)$ as the partition that includes $x$. Let $N(x) = |\mathcal{S}^r(x)|$ and $N = |\mathcal{S}|$.
 Then for any $\kappa \ge 1$,
 \begin{equation}
     \left| \left\{ x ~|~ N(x) \ge \frac{ N }{\kappa \sigma_r}  \right\} \right| \ge \left(1 - \frac{1}{\kappa} + \frac{1}{\kappa \sigma_r}\right)N.
 \end{equation}
\end{lemma}
\begin{proof}
We note that the problem is to show the minimum number of $x$ such that $N(x) \ge N / (\kappa \sigma_r)$. This is equivalent to find the maximum number of $x$ such that $N(x) \le N / (\kappa \sigma_r)$. Since we only have $\sigma_r$ subsets, the maximum can be attained only if for $\sigma_r - 1$ subsets $\mathcal{S}^r$, $|\mathcal{S}^r| = N / (\kappa \sigma_r)$. Otherwise, if for any one of these subsets $|\mathcal{S}^r| < N / (\kappa \sigma_r)$, then it is always feasible to let $|\mathcal{S}^r| = N / (\kappa \sigma_r)$ and the maximum increases. Similarly, if the number of such subsets is less than $\sigma_r - 1$, then it is always feasible to let another subset subject to $|\mathcal{S}^r| = N / (\kappa \sigma_r)$ and the maximum increases. We can then conclude that at most $N(\sigma_r - 1)/(\kappa \sigma_r)$ inputs can have the property $N(x) \le N / (\kappa \sigma_r)$.

\end{proof}
The above lemma basically implies when partitioning $N$ inputs into $\sigma_r$ subsets, a large fraction of the inputs will be assigned to a subset with cardinality at least $N / (\kappa \sigma_r)$. Here $\sigma_r$ is the $r$-covering number and is bounded above based on the property of the covering in the Euclidean space. Apply Lemma~\ref{lemma:bound-partition} to (\ref{eq:final-bound-each-partition}) we then arrive at Theorem~\ref{theorem:error}. 


% There are likely arbitrarily number of possible partitions, but we choose a way that distributes all the inputs as evenly as possible. Strictly speaking, we choose a partition such that it maximizes the cardinality of the subset with the minimum cardinality,
% $$
% \{\mathcal{{S}}_j^r\} = \arg\max_{\{\mathcal{{S}}_j^r\}} ~ \min_j | \mathcal{{S}}_j^r |
% $$



% \begin{remark}[Dependence of $r$]
% \end{remark}
\vspace{1em}
\smallsection{Difference from the Lipschitz bound in generalization theory}
We note that in Theorem~\ref{theorem:error}, the constraint on the local Lipschitz continuity of the hypothesis function is more strict than that is required in typical generalization theory of deep neural networks~\cite{Sokolic2017RobustLM, Bartlett2017SpectrallynormalizedMB}.

\begin{remark}
\label{remark:difference-to-generalization}
% \chengyu{This remark has to be placed after the partition, then we can show why we need more strict Lipschitz given the need for covering the training samples.}
In generalization theory we often require the hypothesis function to be locally Lipschitz continuous around training inputs, such that the difference between the prediction of an unseen input and the prediction of its nearest training input is bounded. However, for learning true label distribution of the training data we need to bound the difference between the predictions of a subset of training inputs. Therefore, our constraint requires the Lipschitz continuity to be established at a larger scale in the input space.

% The distance between two training examples is always larger than the distance between a test example to its closest training example. And Lipschitz in generalization theory requires the Lipschitz on the scale of the distance between a training example and test example. Therefore the Lipschitz here is more strict since a larger scale Lipschitz implies a small scale Lipschitz but not the other way around.

% The approximation error can be arbitrarily large if the Lipschitz is not small. 
\end{remark}

Indeed, we observe from later experiments that our stronger Lipschitz constraint will actually hurt the performance of the teacher on the test set, whereas it can still improve the student performance.
