# Supplementary material for: Toward Student-Oriented Teacher Network Training For Knowledge Distillation
Source: arXiv:2206.06661 source file (2024-05-09)
Supplement: Supplementary file 4 [file 42_proof.tex]

\begin{proof}
Following the proof of Theorem~\ref{theorem:error}, we first partition the augmented training set in a way such that all augmented views of an input $x$ are grouped into the previous subset $\mathcal{S}_j^r$ containing $x$. Therefore we can ensure the covering number will not increase.
% , subsequently the concentration bound will not be looser.
Then we can observe that the differences to the proof of Theorem~\ref{theorem:error} come from two parts. First, in Lemma~\ref{lemma:Lipschitz-true-distribution} we require the true label distributions of all augmented inputs to be close to that of the original input, which induces an additional error term $\|\mathbf{p}^*(A(x)) - \mathbf{p}^*(x)\|$. Second, in the constraint set of minimization problem~(\ref{eq:minimum-partition}) we require the predictions of all augmented inputs to be close to that of the original input, which induces an additional error term $\|\mathbf{f}^*(A(x)) - \mathbf{f}^*(x)\|$. 
% In this scenario, we need to ensure all augmented $x$ has similar true label distribution, then lemma 3.3 still holds. This requires the choice of augmentation operator to not significantly change the true distribution (explains why Mixup/Cutmix) doesn't work. Second, we need to ensure all augmented $x$ has similar model predictions, then lemma 3.4 still holds. This requires consistency regularization between the predictions of augmented samples.
\end{proof}
